# Supplementary material for: Mind Your Credit: Assessing the Health of the Ripple Credit Network
Source: arXiv:1706.02358 source file (2018-03-11)
Supplement: Supplementary file 1 [file appendix-data.tex]

% !TEX root = main.tex

\section{Detailed Ripple Data}

\subsection{Ripple Network}
\label{sec:network-appendix}

\begin{table*}
\begin{tabular}{c | c  c | c  c | c c c c c c c | c |}
& \multicolumn{2}{c |}{\# \accs} & \multicolumn{2}{c| }{\# \links} &  \multicolumn{7}{c|}{Degree Distribution} & Assortativity \\
& Total & Comp  & Total & Comp & Max & Avg & \# Leafs & $>$25\% & $>$50\% & $>$75\% & $>$95\% & \\
\hline
Apr 13 & 1028  & 908  & 1634 & 1554 & 503 & 3.422 & 506 &7 & 64 & 267 & 753 & -0.23\\
Aug 13 & 5693 & 5436  & 8832 & 8679 & 3553 & 3.19 & 3209 &2 & 198 & 1662 & 4569 & -0.31\\
Dec 13 & 15073 & 14744  & 23621 & 23418  & 5870 & 3.17 & 8881 & 3 & 303 & 4450 & 12403 & -0.48\\
\hline
Apr 14 & 24377 & 23855 & 41017 & 40691 & 8194 & 3.41 & 14122 & 4 & 400 & 6622 & 19786 & -0.39\\
Aug 14 & 31784 & 30912  &  56449 & 55839 & 9910 & 3.61 & 18162 & 4 & 460 & 7872 & 25329 & -0.37\\
Dec 14 & 41822 & 40490 & 74538 & 73519 & 11079 & 3.63 & 23914 & 6 & 506 & 10154 & 33139 & -0.35\\
\hline
Apr 15  & 53047 & 51559 & 90974 & 89809 & 14912 & 3.48 & 31352 & 6 & 559 & 13431 & 42579 & \\
Aug 15 & 58530 & 57090 & 101674 & 100621 & 16672 & 3.52 & 34070 & 6 & 580 & 14900 & 47028 & \\
Dec 15 & 63920 & 62211 & 111168 & 109887 & 17455 & 3.53 & 37220 & 6 & 587 & 16130 & 51223 & \\
\hline
Apr 16 & 71231 & 69293 & 119396 & 117916 & 16781 & 3.40 & 42903 & 6 & 588 & 18363 & 57502 &  \\
Aug 16 & 81574 & 79387 & 134073 & 132389 & 16832 & 3.33 & 51057 & 6 & 598 & 20762 & 66149 & \\
Dec 16 & 99565 & 97113 & 174442 & 172547 & 20403 & 3.55 & 58893 & 7 & 634 & 24697 & 79855 & \\
\end{tabular}
\end{table*}
